# Supplementary material for: $^{12}$C(e,e'pN) Measurements of Short Range Correlations in the Tensor-to-Scalar Interaction Transition Region
Source: arXiv:2004.07304 ancillary file (2021-07-25)
Supplement: Supplementary file 1 [file suppl_v1.pdf]

# Tensor-to-Scalar Nucleon-Nucleon Interaction Transitions Mapped by $^{12}\text{C}(e, e'pn)$ Measurements Supplementary Materials

## 1 Neutron identification, detection efficiency, and momentum resolution

In this analysis, we identified neutrons from hits in the SC with no associated charged particle track. Since the charged-particle tracking efficiency in CLAS is not 100%, some charged particles can be misinterpreted as neutral particle hits. For our analysis, due to the low number of recoil neutrons and the higher charged-particle multiplicity, we needed to veto this background. We developed a veto algorithm that used drift chamber (DC) information to remove hits in the SC that could plausibly have come from a charged particle whose track was not reconstructed.

The efficiency for neutrons interacting in the SC is on the order of a few percent. We characterized this efficiency using the  $d(e, e'p)n$  reaction. The veto algorithm and neutron efficiency study are described in the following sections.

### 1.1 Veto Algorithm

Our veto algorithm makes use of SC and DC hit information to identify neutral candidates and veto those that could have come from a charged particle.

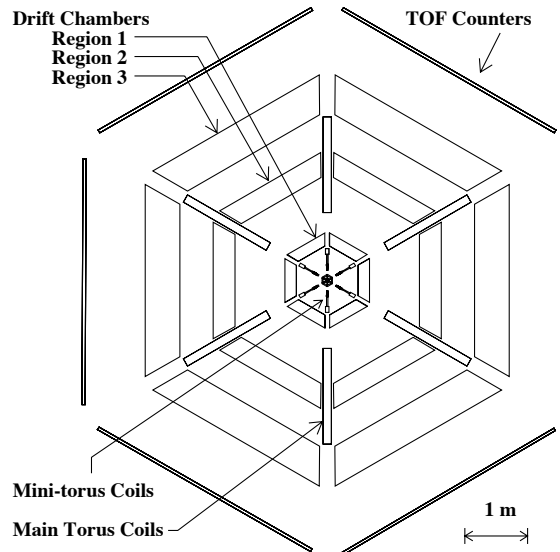

Figure S1: Schematic of CLAS viewed down the beamline, taken from [1]

The CLAS drift chambers [2] were grouped into three regions, with region 1 closest to the beamline, and region 3 farthest from the beamline, as can be seen in the schematics in Figs. S1 and S2. Each region was

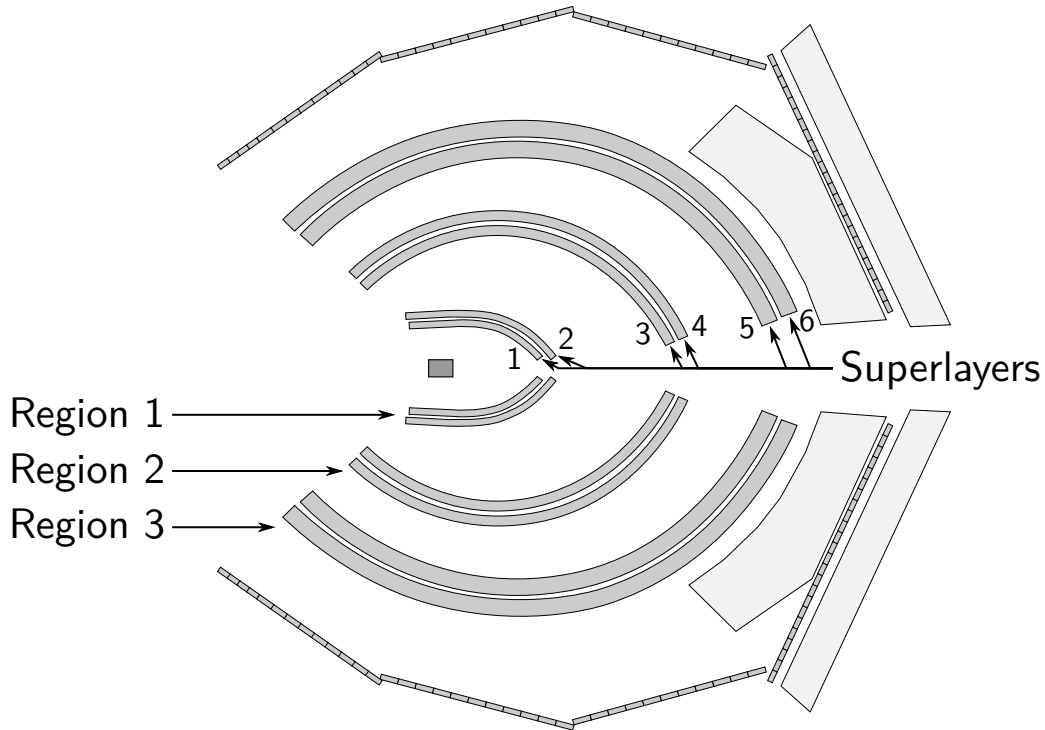

Figure S2: Schematic of CLAS viewed from above

comprised of two superlayers, numbered 1 through 6, with 1 closest to the beamline and 6 furthest from the beamline. The wires in alternating superlayers were offset by a  $6^\circ$  stereo angle to provide information about the track azimuth as well as polar angle.

Individual superlayers were comprised of hexagonal drift cells, arranged in six layers, with the exception of superlayer 1, which had four layers (see Fig. S3). A track passing through the drift chambers would intersect 34 layers.

The first step in the algorithm is to identify signals in the drift chambers from charged particles, even if these CLAS tracking algorithm failed to identify a track. CLAS tracking algorithms require DC hits in all 6 superlayers in order to form a track. If a track fails to register a signal in any superlayer, the track reconstruction will fail. Our algorithm to identify charged particle signatures needs to be robust to this possibility, while also being able to point where charged particle trajectory intersected the SC.

For these reasons, our algorithm only considers hits in DC Region 3, clusters them into partial tracks, which we call “tracklets.” Region 3 is outside of the CLAS toroidal magnetic field, and so charged particle trajectories are straight lines through the region, all the way to the SC. By fitting a straight line to a tracklet, we can project this line to the SC and get a good idea of the charged-particle hit position and exclude nearby neutral candidates. We can form a tracklet with a minimum of two DC hits.

For each tracklet, we define an exclusion region around its SC hit position using the sector coordinates  $X$ ,  $Y$ , and  $Z$  of the SC hit. Nominally the exclusion region was chosen to be  $\Delta X = 50$  cm,  $\Delta Y = 50$  cm, and  $\Delta Z = 50$  cm. We studied the systematic effects of varying the exclusion window size, and these studies are described below.

Once we have assembled a list of tracklets as well as their combined exclusion regions, we loop over the hits in the SC, classifying them as either neutral candidates or as charged background. The flowchart of the algorithm is shown in Fig. S4. First, we veto the hit if it has already been assigned to a valid charged-particle track. Next, we veto the hit if its position is within the exclusion region of any tracklets. The third step in the algorithm is to merge any neutral candidates that are close together. The rationale of this merge step is that SC hits close together are likely caused by the same particle. We defined “close together” using a merging window based on time difference and SC paddle difference. The nominal window was chosen to be  $\Delta \text{Paddle} < 2$  and  $\Delta t < 5$  ns, and effect of changing the merging window was also studied. When merging

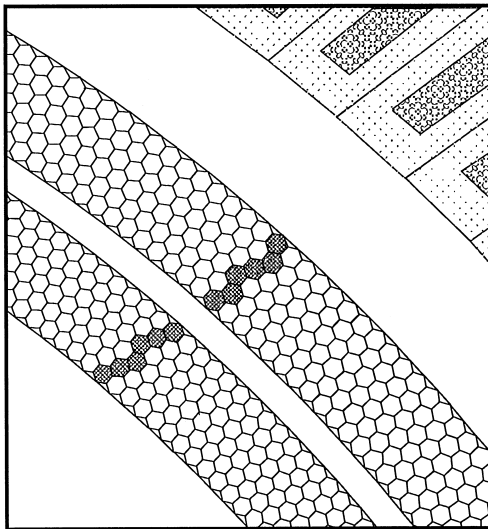

Figure S3: A schematic showing the drift cells in region 3, taken from [2]

two neutral candidates, the hit position and time were taken from the earlier hit.

Figs. S5, S6, and S7 show illustrations of how the veto algorithm works in different scenarios. The illustrations show cross sections of a CLAS sector, along with DC hits (red squares) and SC hits (circles), tracklet fits (dashed blue lines), exclusion regions (blue circles), and merging windows (green circles). Neutral candidates The illustrations do not portray any specific events in particular, but provide some visual clarification of the workings of the veto algorithm.

### 1.1.1 Window Size Studies

The sizes of the exclusion region and merging window were varied and the spread in results was included as a systematic uncertainty on the final result. The values used in this study are shown in Table S1. In the  $x$  and  $z$  direction we wanted to choose as a nominal cut a range that is large enough to exclude, for each hit, the hit paddle as well as the centers of the two neighboring paddles on either side. This minimum distance varies between 15 cm and 45 cm depending on the widths and orientations of the paddles. Therefore we conservatively selected 50 cm for the nominal exclusion window in the  $x$  and  $z$  directions. In the  $y$  direction (along the length of the paddles), we needed a different rationale. Fig. S8 shows the difference in position between the hit in the bar and reconstructed hit position for the closest charged particles to this hit. We chose to conservatively exclude 4 times the FWHM of this distribution, which corresponds to  $\approx \pm 50$  cm.

The size of the exclusion range impacts the eventual neutron detection efficiency. We tested different values for sizes of the exclusion windows in all three directions (shown in Table S1) and determined that the change in the neutron efficiency is small (see Fig. S26 in section 1.2.3).

Table S1: The values defining the exclusion region ( $\Delta X$ ,  $\Delta Y$ ,  $\Delta Z$ ) and mergin window ( $\Delta Paddle$ ,  $\Delta t$ ) used in the sensitivity study

| Condition       | Nominal Value | Values considered                |
|-----------------|---------------|----------------------------------|
| $\Delta X$ [cm] | 50            | 40, 50, 70, 80, 90               |
| $\Delta Y$ [cm] | 50            | 50, 100, 120, 140, entire paddle |
| $\Delta Z$ [cm] | 50            | 40, 50, 70, 80, 90               |
| $\Delta Paddle$ | $< 2$         | $< 2$ , $< 3$                    |
| $\Delta t$ [ns] | 5             | 2, 5, 10, no requirement         |

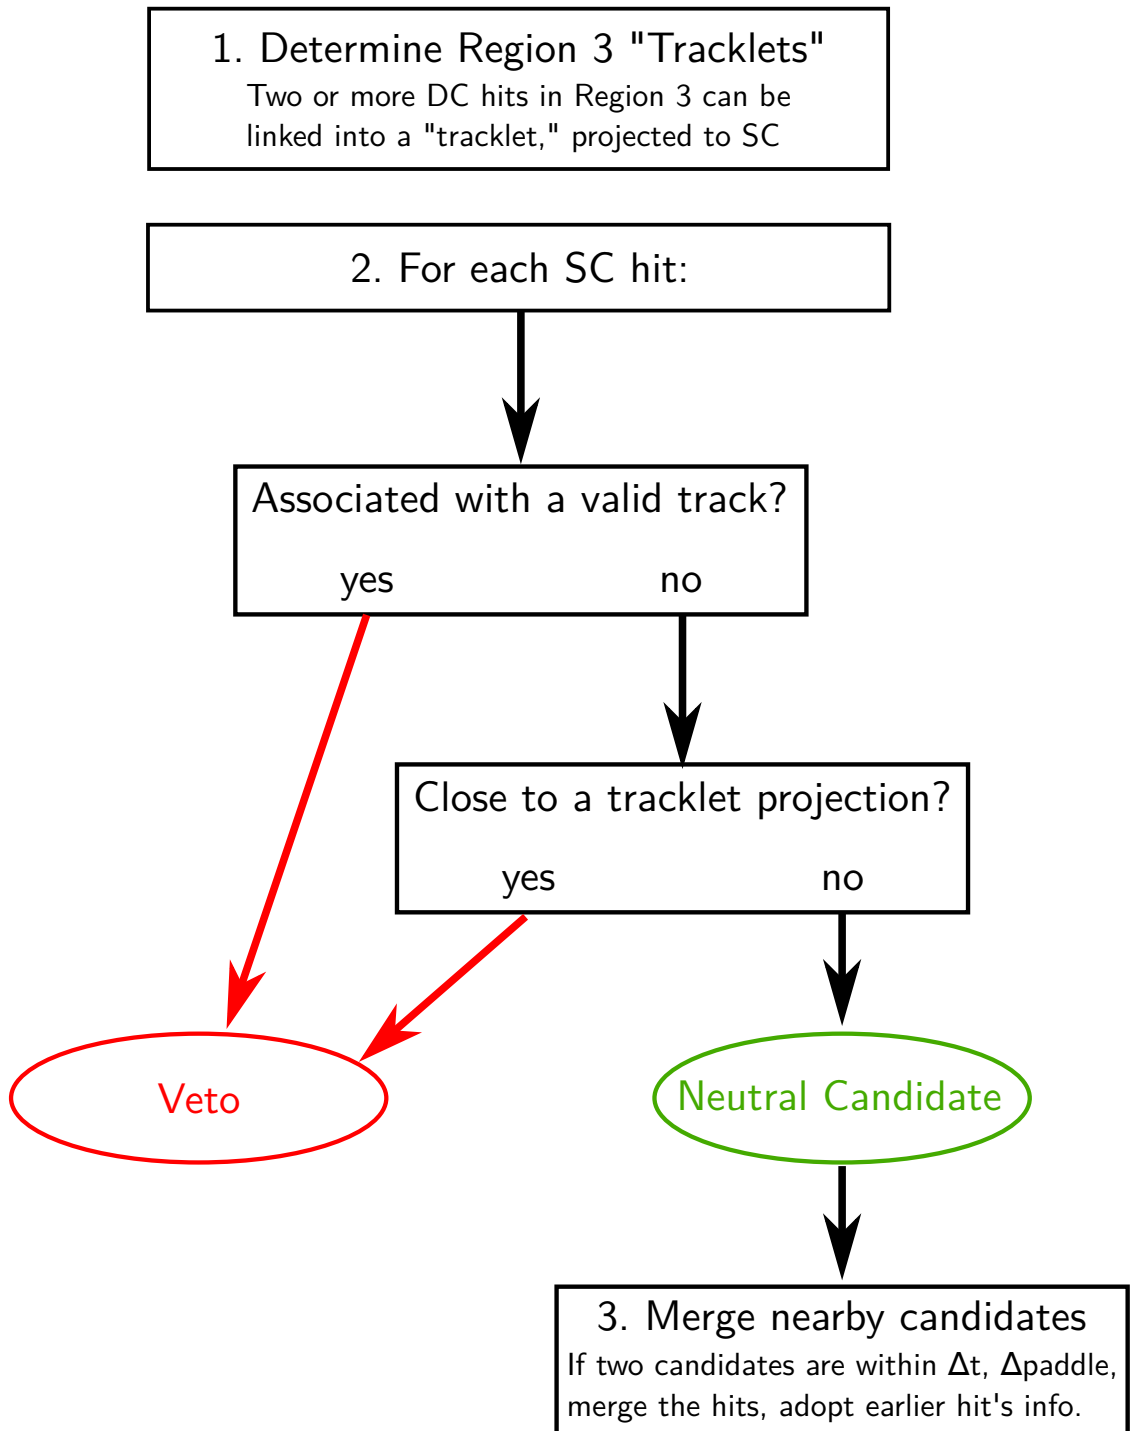

Figure S4: A schematic view of the charged-particle veto algorithm

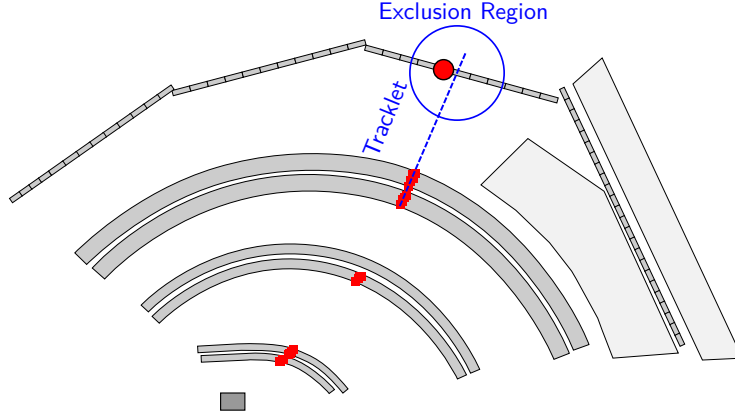

Figure S5: In this event, there was an out-bending charged particle that could not be tracked due to hits missing in the outer superlayer of Region 2. However, a tracklet could be fit to the Region 3 hits, which successfully vetoed the SC hit within the exclusion region.

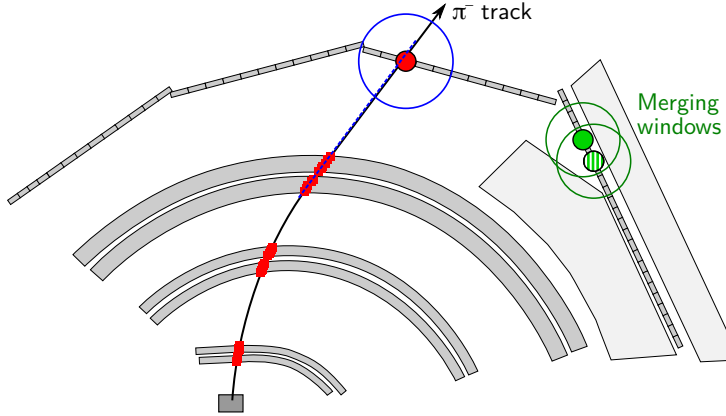

Figure S6: In this event, there were three SC hits. One was associated with a successfully tracked  $\pi^-$ , and therefore vetoed. The other two hits were classified as neutral candidates, but since they fall within the merging windows, they were merged, taking the time and position information from the earlier hit (solid green).

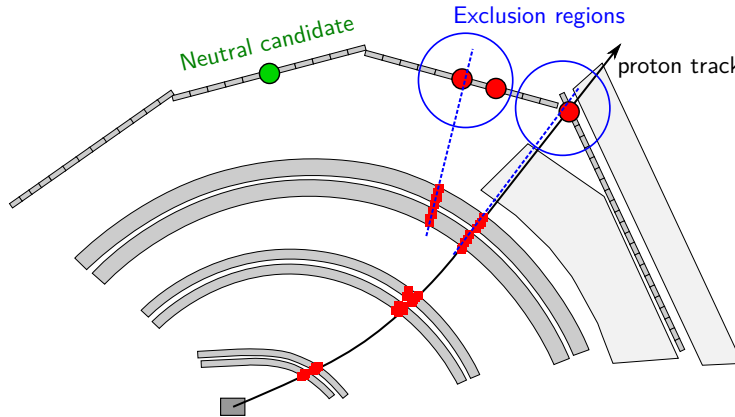

Figure S7: In this event, there were two closely overlapping out-bending particles, of which only one was successfully tracked. Its assigned SC hit was vetoed. The additional region 3 hits were sufficient to fit a tracklet, whose exclusion region encompassed two SC hits, which were therefore both vetoed. A fourth SC hit at back angles was outside any exclusion region, and so was classified as a neutral candidate.

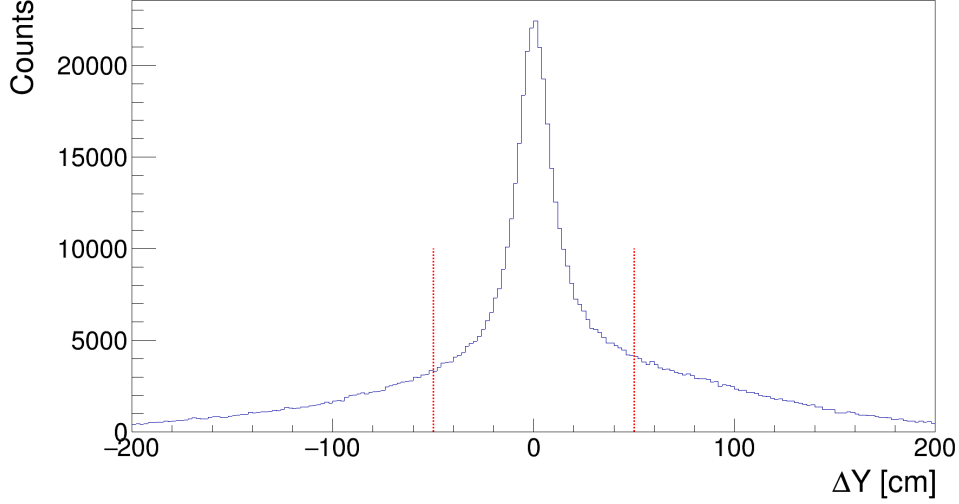

Figure S8: Difference in y-axis (along the bars) between charge hit position to neighbor reconstructed charge hits. See text for details.

### 1.1.2 Veto Efficacy

The effect of the veto algorithm can clearly be seen in Fig. S9, which shows the SC energy deposition of neutron candidates without (red) and with (blue) the veto algorithm. Neutron candidates have been selected from neutral candidates by requiring a time-of-flight per meter between 4 and 12 ns/m (i.e.,  $0.28 < \beta < 0.83$ , eliminating gammas), making a fiducial requirement that the SC hit be at least 10 cm away from the paddle edges. The red histogram was produced by eliminating only SC hits assigned to a valid track. The blue histogram uses the full veto algorithm, including the exclusion regions around Region 3 tracklets. Without the veto algorithm, the red histogram shows a peak at approximately 12 MeV, which corresponds to minimum-ionizing particles (MIPs). By using the veto algorithm, the blue histogram shows that this MIP peak is effectively eliminated.

## 1.2 Neutron Efficiency

The results of this analysis require characterizing the neutron detection efficiency. This was studied using data from the deuterium target, from which we could exploit the over-constrained  $d(e, e'p)n$  reaction. By selecting events  $d(e, e'p)n$  using missing mass, and by determining the likely neutron momentum direction using missing momentum, we could determine the efficiency of the SCs for detecting the neutron.

### 1.2.1 $d(e, e'p)n$ Event Selection

EG2 used a dual target system in which both a liquid deuterium cell and a solid target foil were placed in the beamline simultaneously. The first step in event selection was to require that the electron vertex lie within the liquid cell region, i.e.,  $-31.1 < z_e < -29.5$  cm. We also require that the proton and electron have a small vertex difference, i.e.,  $|z_e - z_p| < 0.8$  cm ( $\sim 2\sigma$ ). These cuts are illustrated in Fig. S10.

After making vertex cuts, we examined the missing mass distribution, shown in Fig. S11. We define missing mass,  $m_{\text{miss}}$ , as the mass of the undetected system, given by

$$m_{\text{miss}}^2 \equiv m_d^2 + m_p^2 - Q^2 + 2m_d(\omega - E_p) - 2\omega E_p + 2\vec{p}_p \cdot \vec{q}, \quad (1)$$

where  $m_d$  is the mass of the deuteron,  $m_p$  is the mass of the proton,  $p_p$  is the momentum of the detected proton,  $E_p = \sqrt{p_p^2 + m_p^2}$ , and  $(\omega, \vec{q})$  are the energy and momentum transferred by electron such that  $Q^2 = q^2 - \omega^2$ . Fig. S11 shows a clear peak at approximately the mass of the neutron, as well as a substantial background.

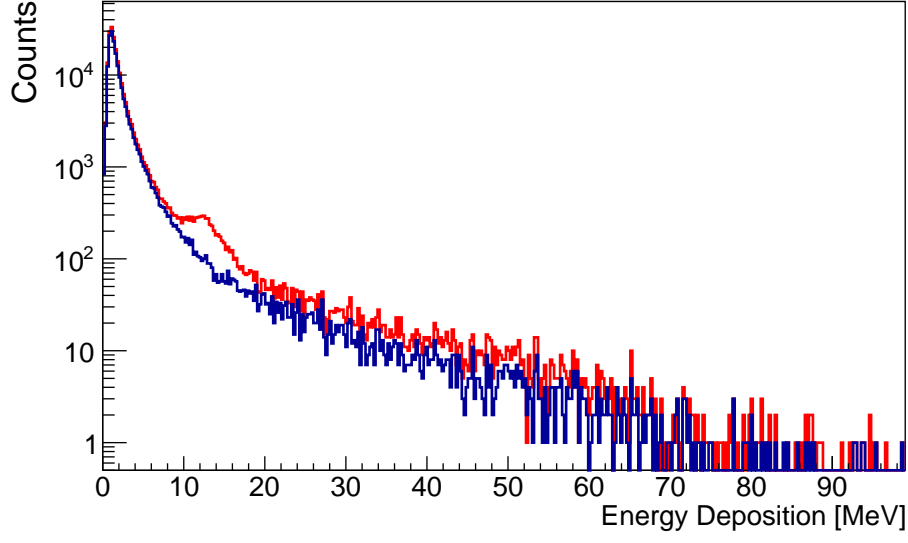

Figure S9: The energy deposition of neutral candidates without (red) and with (blue) the veto algorithm. Without the veto, there is a clear peak at  $\approx 12$  MeV, corresponding to a MIP-like energy deposition. The veto algorithm eliminates this MIP contribution. See text for additional details.

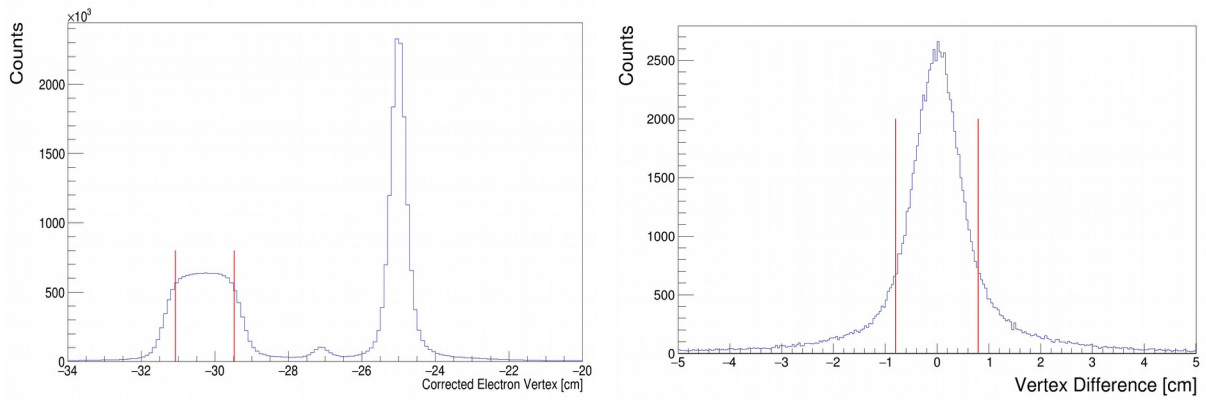

Figure S10: Left: Electrons were selected so that their vertex corresponded to the liquid deuterium cell. Right: The proton vertex was required to be within 0.8 cm ( $\sim 2\sigma$ ) of the electron vertex.

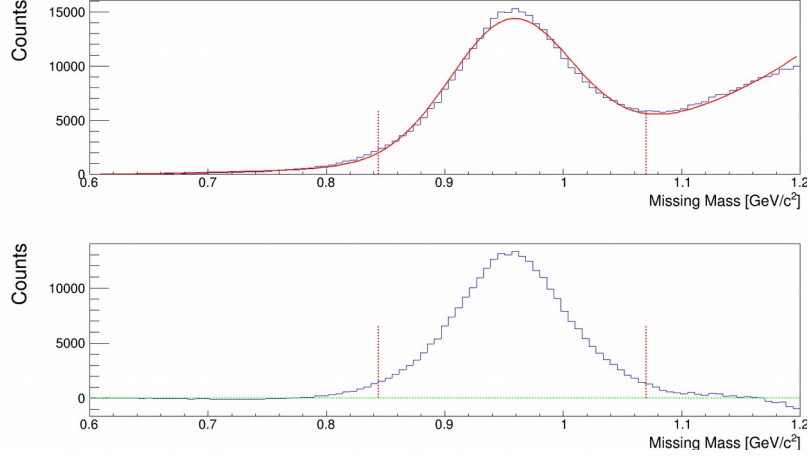

Figure S11: Top: The missing mass distribution after vertex cuts. Bottom: The background-subtracted missing mass distribution.

93 The background was well-described using an empirical fit to the side-bands. The fit function was parametrized  
 94 byx

$$f = e^{(a+bx)} + c, \quad (2)$$

95 where  $a$ ,  $b$ , and  $c$  are the free parameters.

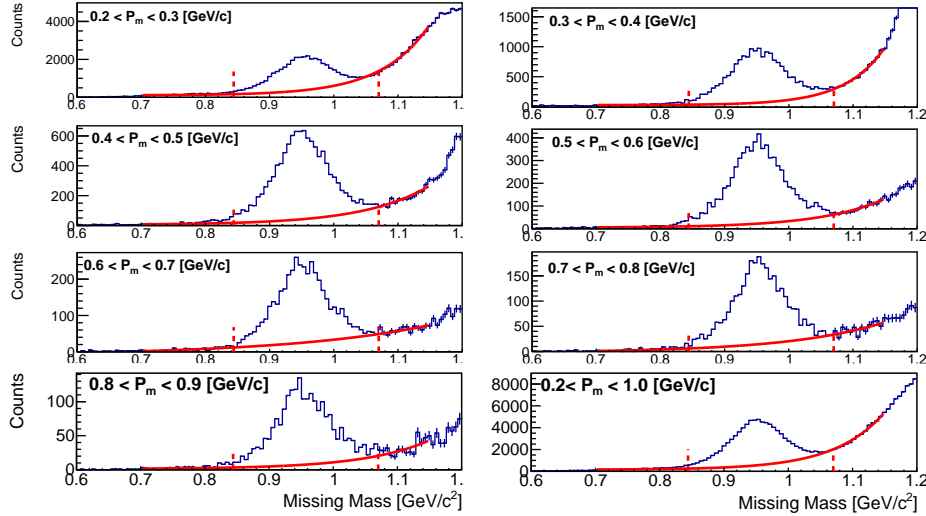

Figure S12: The missing mass distribution and background fits for eight regions of missing momentum.

96 The width of the neutron peak in the missing mass distribution comes from resolution effects and could  
 97 be heavily kinematics-dependent. We examined the dependence on missing momentum by looking at the  
 98 distribution in eight different bins of missing momentum in the range of interest:  $0.2 < p_{\text{miss}} < 1.0$  GeV/c,  
 99 shown in Fig. S12. This allowed us to fit the widths and background levels for each individual  $p_{\text{miss}}$  region.  
 100 We fit the background-subtracted spectra with a Gaussian and placed a  $\pm 1\sigma$  cut around the peak. We also  
 101 accounted for the background remaining under the peak, as described below.

102 In order for a  $d(e, e'p)n$  event to be a useful probe of the SC efficiency, the neutron needed to have passed  
 103 through the SC. The neutron direction, however, was determined from the missing momentum, which in  
 104 turn was limited by the electron and proton resolutions. An additional fiducial cut on the inferred neutron

direction was needed to avoid edge cases in which the neutron missed the SC, even though the inferred direction pointed toward the SC. Such edge cases would cause an underestimate of the efficiency.

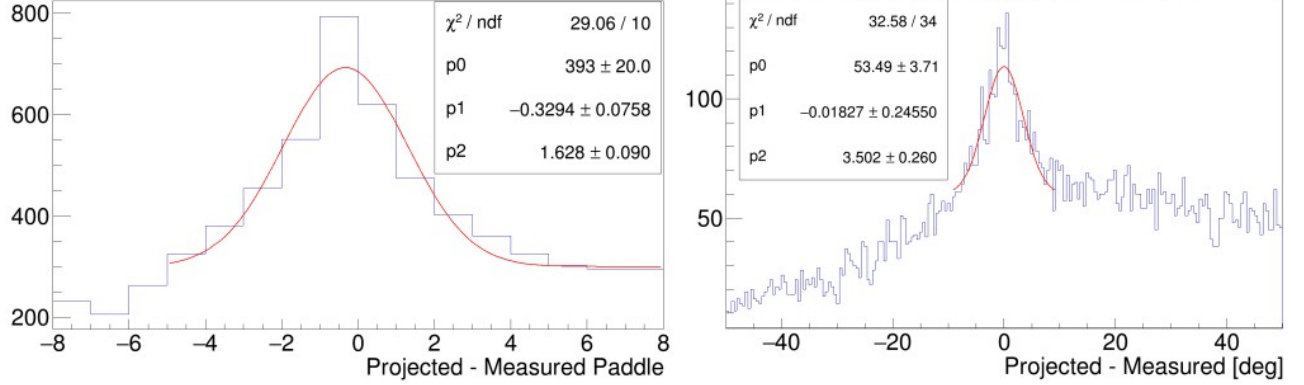

Figure S13: The difference between the projected and measured neutron hits in the in-plane direction. Left shows  $\Delta$  Paddle, while Right shows the same data converted to degrees. These plots use the following  $d(e, e'pn)$  selection cuts: electron vertex, vertex difference, missing mass,  $0.3 < p_{\text{miss}} < 1.0$  GeV/c,  $E_{\text{dep}}^{\text{SC}} > 7$  MeV, and removing the outer 10 cm of each SC paddle as a fiducial cut.

To estimate the neutron direction resolution, we compared the difference between the projected and measured neutron hits both in the in-plane ( $\Delta$  Paddle) and out-of-plane ( $\Delta\phi$ ) directions. Events passing  $d(e, e'p)n$  cuts that also had a neutral-candidate SC hit with  $> 7$  MeV of energy deposition were selected as  $(d, e'pn)$  events. The outer 10 cm of each SC paddle were excluded as a fiducial cut. Gaussian fits with a constant background indicated a in-plane resolution of 1.6 paddles, or approximately  $3.5^\circ$  (Fig. S13) and an out-of-plane resolution of  $2.8^\circ$  (Fig. S14).

We designed a neutron direction fiducial cut with the goal of excluding at least  $2\sigma$ -worth of neutron resolution from the edges of the SC paddles. First, we used the scintillator geometry information from the ToF NIM paper [3] to estimate the coordinates for the edges of each scintillator paddle. As a safety margin, we eliminated 10 cm from the end of each paddle. Then, we fit these truncated positions with a parameterized function, given by:

$$\phi_{\text{limit}}(\theta) = a \cdot \theta^b + c \cdot \theta^d. \quad (3)$$

Given this parameterization of the SC edges in  $\theta, \phi$  space, we required that the inferred neutron direction be greater than  $6^\circ$  and 4 paddles from this edge.

Fig. S15 illustrates the parameterization of Eq. 3 and the effect of the fiducial cut.

In summary, here are the event selection criteria for  $d(e, e'p)n$  events:

- Electron vertex:  $-31.1 < z_e < -29.5$  cm,
- Vertex difference:  $|z_e - z_p| < 2\sigma$  cm,
- Missing momentum:  $0.3 < p_{\text{miss}} < 1.0$  GeV/c,
- Missing mass:  $|\Delta m_{\text{miss}}| < 1\sigma$ , as a function of  $p_{\text{miss}}$ ,
- Neutron direction fiducial cut: 6 cm out-of-plane and 4 paddles in-plane

### 1.2.2 $d(e, e'pn)$ Event Selection

$d(e, e'pn)$  events were selected from the set of  $d(e, e'p)n$  by additionally requiring a unvetoes neutron candidate hit in the SC, matching several kinematic conditions. We required the hit to be within a “neutron fiducial region,” excluding the outer 10 cm of each side of each SC paddle. We placed a cut on the SC energy deposition to help reduce the low-energy background. The placement of this threshold cut is a compromise between the

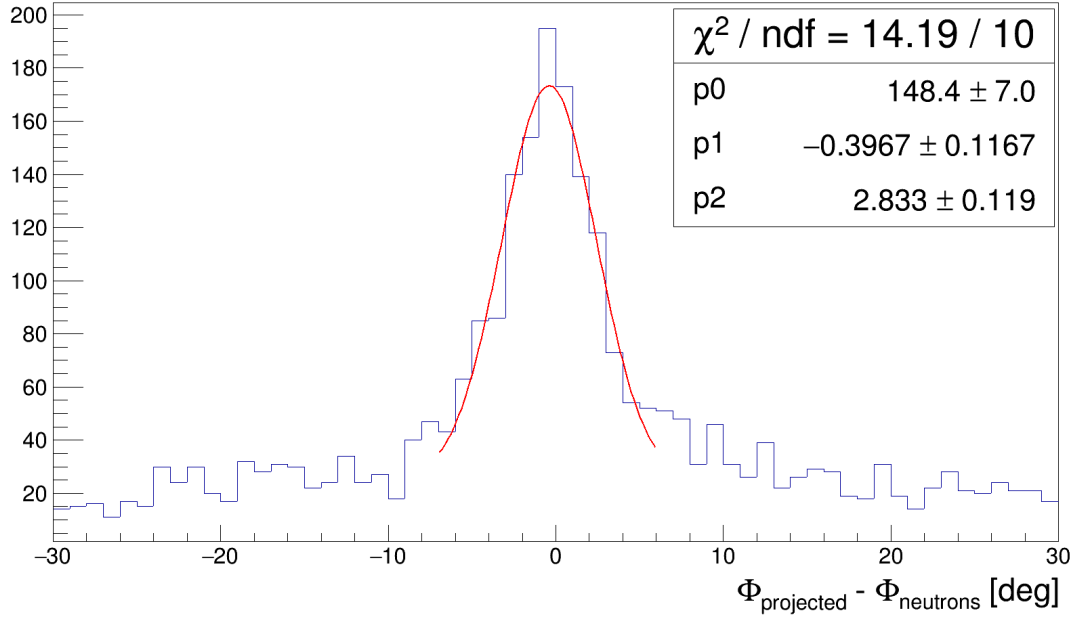

Figure S14: The difference between the projected and measured neutron hits in the out-of-plane direction. The same  $d(e, e'pn)$  event selection cuts have been applied as in Fig. S13.

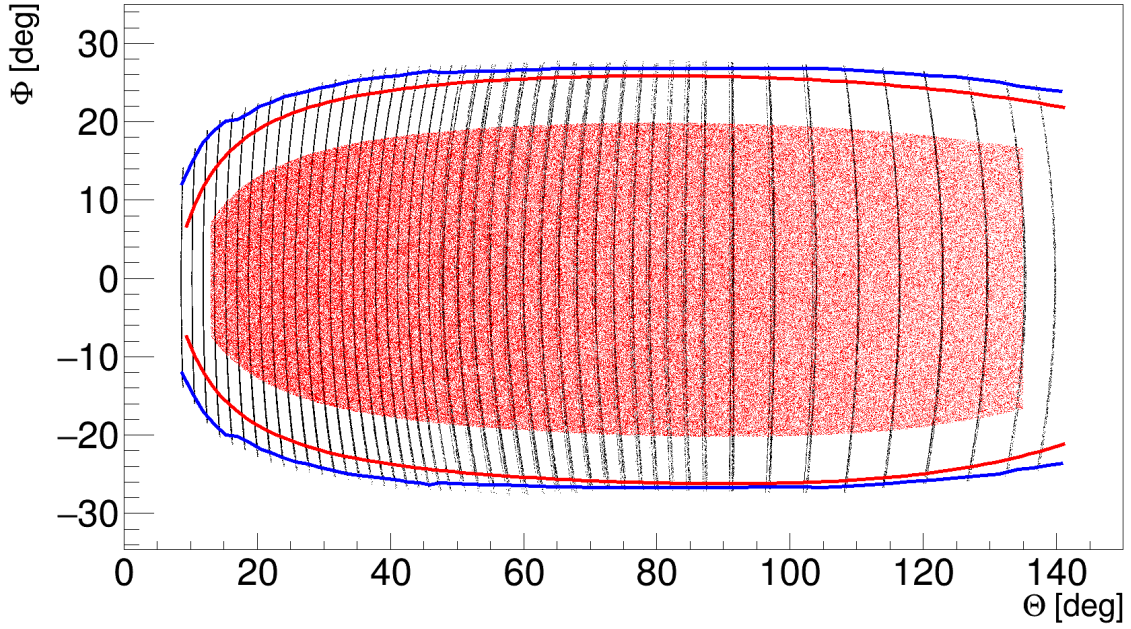

Figure S15: The SC paddle acceptance in  $\theta, \phi$  space. The blue line represents the geometrical limit of the SC based on the data in Ref. [3]. The red line shows the parameterization of Eq. 3. The difference is largely the result of the 10 cm safety margin applied when fitting the data. The red dots show the inferred neutron directions for events passing  $d(e, e'p)n$  criteria as well as the fiducial requirement of being greater than  $6^\circ$  and 4 paddles from the red line. The black dots show the reconstructed positions of neutral candidate SC hits, which are assigned to the centerline of their respective paddles.

goals of high efficiency (favoring a lower cut) and minimal background (favoring a higher cut). We chose a nominal value of 8 MeV. We also varied this cut between 4 and 10 MeV as a sensitivity study. Furthermore, as exclusivity requires that the neutron emerge in the opposite direction to the missing momentum, we required that the cosine of the opening angle, defined by the angle between  $\vec{p}_{\text{miss}}$  and the neutron momentum vector  $\vec{p}_n$ , be smaller than  $-0.95$ .

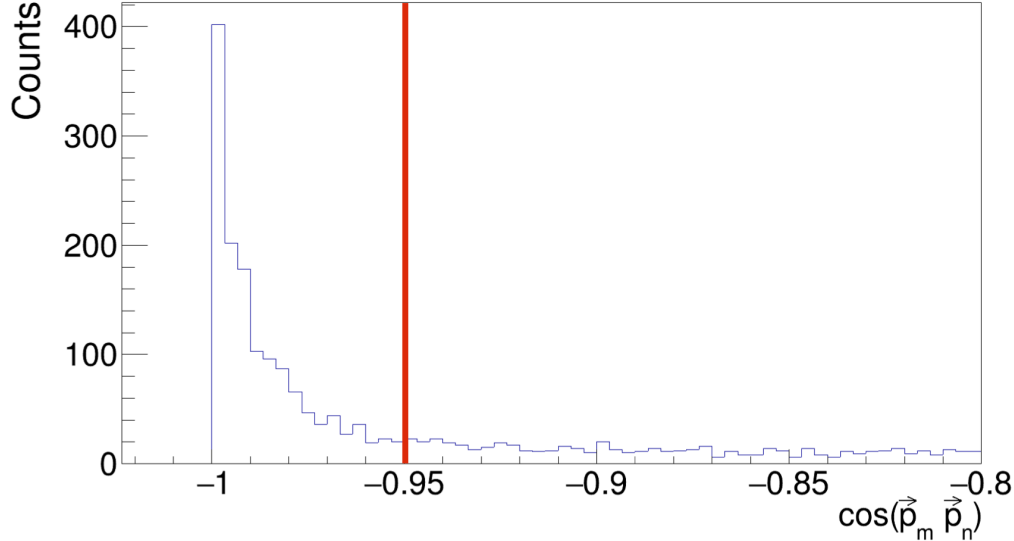

Figure S16: The opening angle distribution for  $d(e, e'pn)$  events passing the  $d(e, e'p)n$  event selection criteria, neutron fiducial cut, and the  $E_{\text{dep.}}^{\text{SC}}$  cuts. The distribution peaks at  $-1$ , as expected from exclusivity. We further excluded events with  $\cos(\vec{p}_m \cdot \vec{p}_n) > -0.95$ , as marked by the red vertical line.

The reconstructed opening angle in  $d(e, e'pn)$  events passing both the  $d(e, e'p)n$  event selection and the neutron SC energy deposition cut are shown in Fig. S16. The distribution is peaked at  $-1$ , as one would expect from exclusive events. We further studied this distribution as a function of  $p_{\text{miss}}$ , shown in Fig. S17, which demonstrated that a  $-0.95$  cut is suitable for the entire  $p_{\text{miss}}$  range.

Next, we considered the timing information of the neutron hit. To eliminate off-time background, we required that the neutron hit arrive in a time-of-flight window of interest between 22 and 70 ns. The lower limit (shorter time-of-flight) was chosen to remove the gamma contamination. As shown in Fig. S18, the gamma peak position plus  $3\sigma$  is at  $16.7 + 3 \cdot 1.7 \approx 22$  ns. The upper limit (longer time-of-flight) was chosen to remove the random coincidence background corresponding to momenta below our region of interest, i.e.,  $p_n < 200$  MeV/c.

Fig. S19 shows the time-of-flight distribution for neutrons, for bins in  $p_{\text{miss}}$ . From exclusivity, the neutron momentum magnitude should be equal to  $p_{\text{miss}}$  (see correlation in Fig. S20). As expected the neutron time-of-flight decreases with  $p_{\text{miss}}$ .

Given  $p_{\text{miss}}$ , and the neutron path length,  $L_n$ , we can predict the neutron time-of-flight. We define the difference between the measured neutron time-of-flight and the expected time-of-flight as the “corrected time of flight,” given by the following equation:

$$T_{\text{corr}} \equiv T_{\text{SC}}^n - \frac{L_n}{c} \sqrt{1 + \frac{m_n^2 c^2}{p_{\text{miss}}^2}}. \quad (4)$$

Fig. S21 shows the corrected time-of-flight distribution by  $p_{\text{miss}}$ . The distributions peak around zero, as expected. The  $T_{\text{corr}}$  resolution changes with missing momentum due to the different regions in class in which the neutrons are detected. For example, the backward angle scintillators are larger and read out in pairs, leading to reduced pathlength resolution. To remove non-exclusive background, we apply a  $2\sigma$  corrected time-of-flight cut as a function of  $p_{\text{miss}}$ .

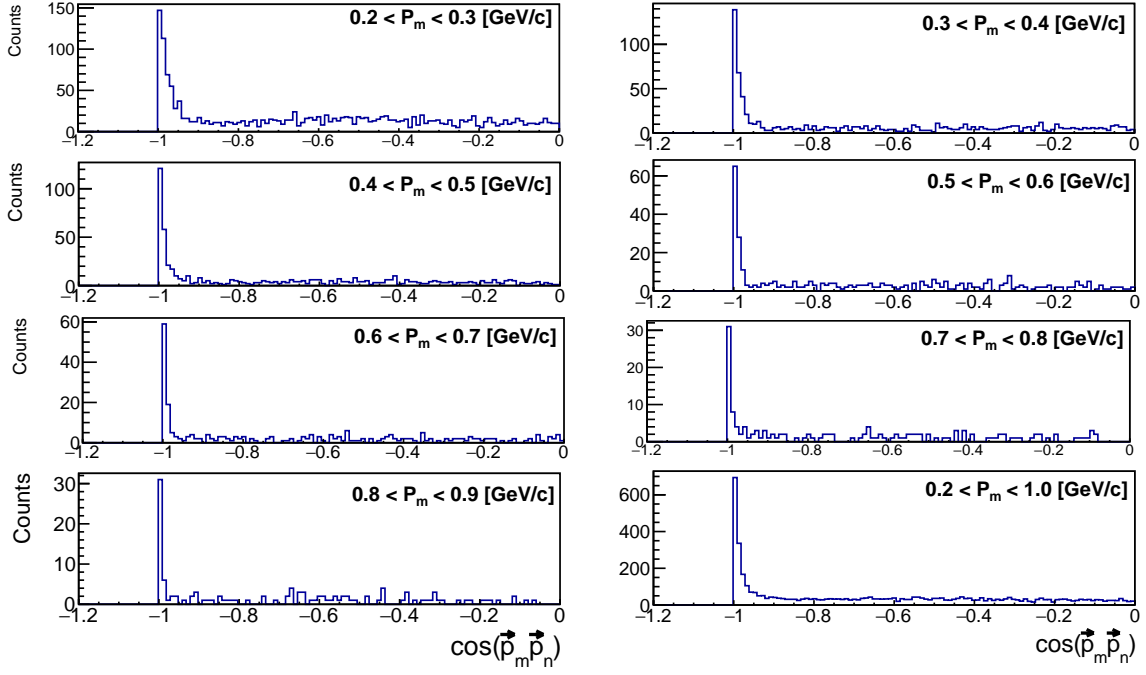

Figure S17: The opening angle distribution for  $d(e, e'pn)$  events passing the same criteria as in Fig. S16, in eight regions of  $p_{\text{miss}}$ . The opening angle resolution improves at higher  $p_{\text{miss}}$ .

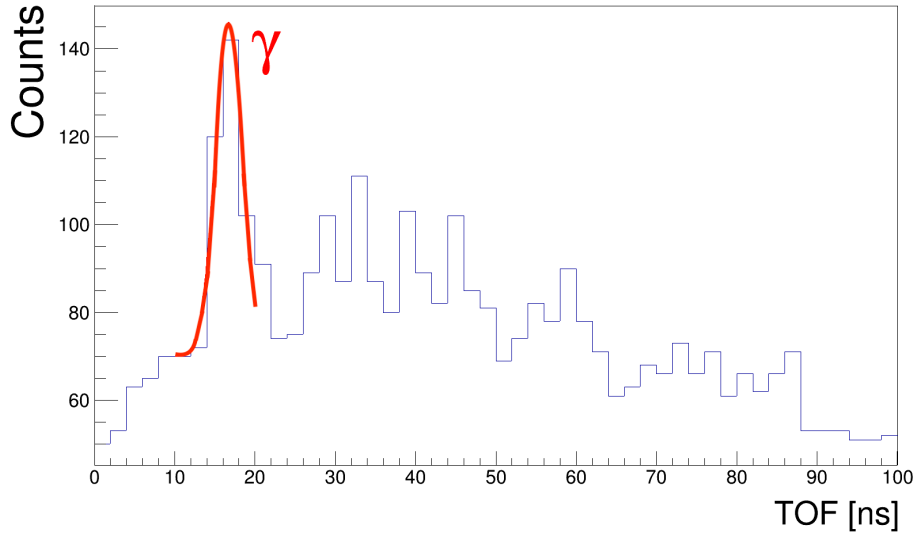

Figure S18: The time-of-flight distribution for  $d(e, e'pn)$  events passing the  $d(e, e'p)n$  selection criteria, neutron fiducial and energy deposition cuts. The gamma peak has been fit with a Gaussian plus constant background.

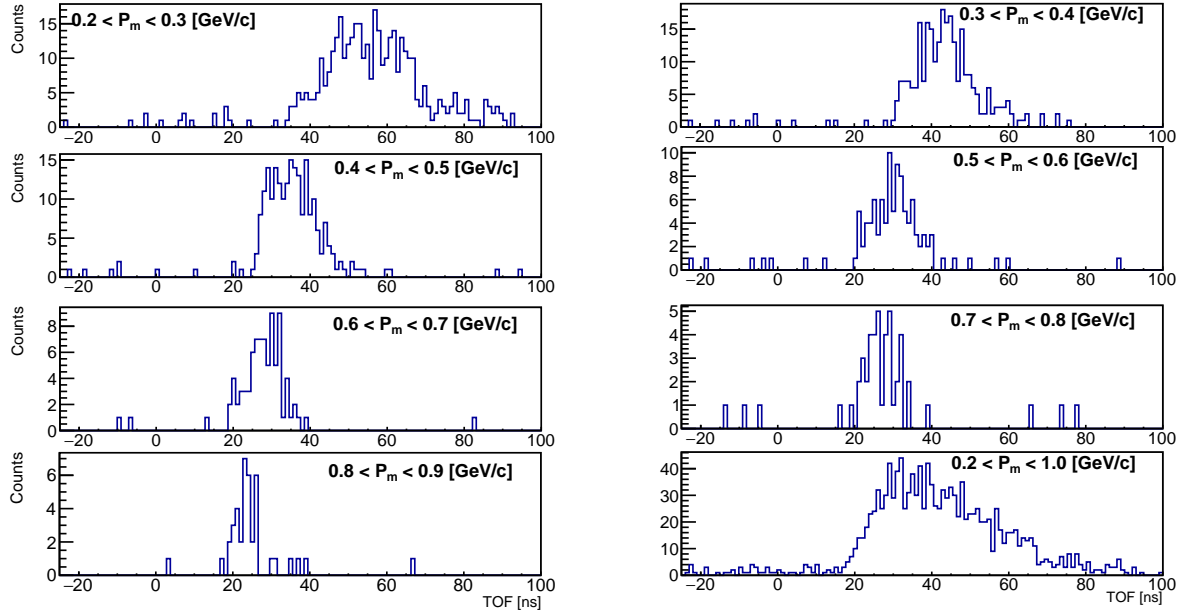

Figure S19: The neutron time-of-flight distribution for  $d(e, e'pn)$  events passing the  $d(e, e'p)n$  selection criteria, neutron fiducial, energy deposition, and opening angle cuts. As expected from exclusivity, the time-of-flight decreases with missing momentum.

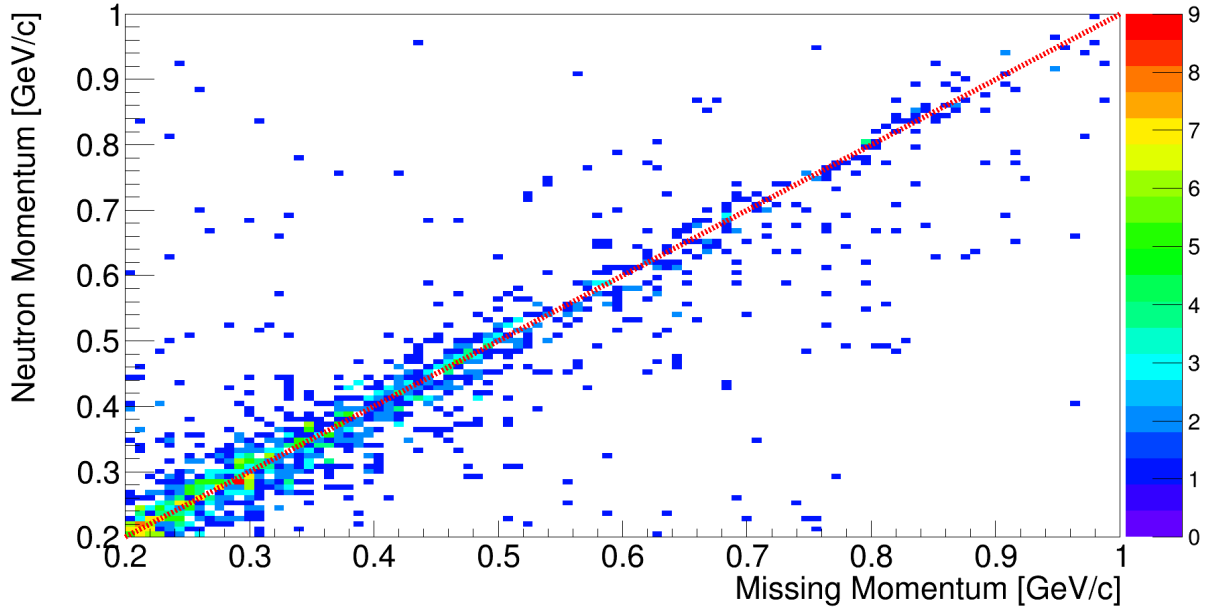

Figure S20: The neutron momentum (determined from time-of-flight) as a function of  $p_{\text{miss}}$  for events passing the  $d(e, e'p)n$  selection criteria, neutron fiducial, energy deposition, and opening angle cuts.

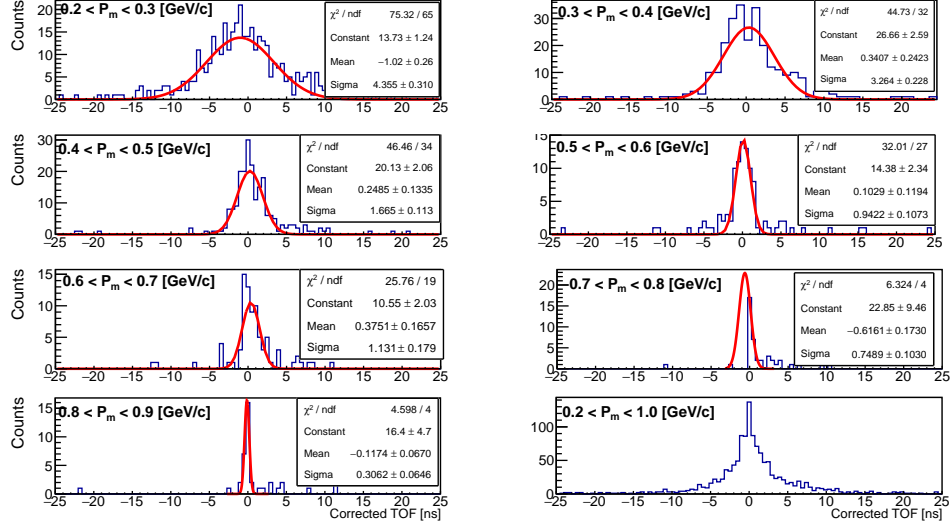

Figure S21: The corrected neutron time-of-flight distribution for  $d(e, e'pn)$  events passing the  $d(e, e'p)n$  selection criteria, neutron fiducial, energy deposition, and opening angle cuts.

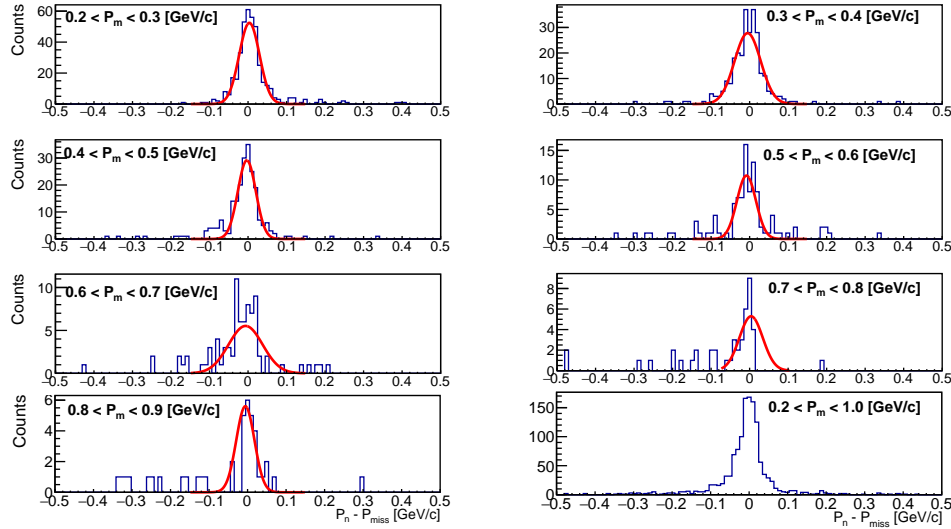

Figure S22: The neutron momentum difference (Eq. 5) in units of GeV/c, for regions of  $p_{miss}$ .

Table S2: Neutron resolution parameters

| $p_{\text{miss}}$ | Range    | $\langle p_n \rangle$ [GeV/ $c$ ] | $\sigma_{p_n}$ [GeV/ $c$ ] | $\sigma_{p_n}/\langle p_n \rangle$ |
|-------------------|----------|-----------------------------------|----------------------------|------------------------------------|
| 0.2–0.3           | GeV/ $c$ | 0.25                              | 0.036                      | 14.4%                              |
| 0.3–0.4           | GeV/ $c$ | 0.35                              | 0.040                      | 11.5%                              |
| 0.4–0.5           | GeV/ $c$ | 0.45                              | 0.032                      | 7.1%                               |
| 0.5–0.6           | GeV/ $c$ | 0.55                              | 0.030                      | 5.5%                               |
| 0.6–0.7           | GeV/ $c$ | 0.65                              | 0.036                      | 5.5%                               |
| 0.7–0.8           | GeV/ $c$ | 0.75                              | 0.029                      | 3.9%                               |
| 0.8–0.9           | GeV/ $c$ | 0.85                              | 0.024                      | 2.8%                               |
| 0.2–1.0           | GeV/ $c$ | 0.40                              | 0.044                      | 11.0%                              |

Similar to corrected time-of-flight, we can define the neutron momentum difference

$$\Delta p_n = \frac{m_n L_n}{\sqrt{T_{\text{SC}}^2 c^2 - L_n^2}} - p_{\text{miss}}, \quad (5)$$

shown in Fig. S22. We determine the neutron momentum resolution by fitting these distributions, with the results given in Table S2.

To summarize, our  $d(e, e'pn)$  event section cuts are:

- Neutron fiducial cuts,
- $E_{\text{dep}}^{\text{SC}}$  cut,
- Opening angle between  $\vec{p}_n$  and  $\vec{p}_{\text{miss}}$  satisfying  $\cos \theta < -0.95$ ,
- Time-of-flight within expected window:  $22 < T_{\text{SC}}^n - t_0 < 70$  ns,
- Corrected time-of-flight within  $\pm 2\sigma$ , as a function of  $p_{\text{miss}}$ .

We can test the effectiveness of these cuts by looking at the missing mass distribution (calculated using electron and proton information) after making neutron cuts (Fig. S23). After making  $d(e, e'pn)$  selection cuts, the missing mass distribution is peaked around the neutron mass, and most of the non-exclusive background has been eliminated.

### 1.2.3 Efficiency Results

To determine the efficiency as a function of  $p_{\text{miss}}$ , our proxy for neutron momentum, we divide the  $d(e, e'pn)$  yield by the background-subtracted  $d(e, e'p)n$  yield. The results are shown in Fig. S24 for different values of the energy deposition cut. Depending on the value used, the efficiency for neutrons with momenta greater than 400 MeV/ $c$  is approximately 4–5%.

We parameterized the neutron efficiency as a function of momentum with a three-parameter piece-wise function,

$$\epsilon(p_n) = \begin{cases} \epsilon_0 + bp_{\text{miss}} & p_n < \frac{\epsilon_{\text{max}} - \epsilon_0}{b} \\ \epsilon_{\text{max}} & p_n \geq \frac{\epsilon_{\text{max}} - \epsilon_0}{b} \end{cases}, \quad (6)$$

with a linear region at low momentum joined continuously to a plateau at high momentum. We fit the parameters to the efficiency data using missing momentum as a proxy for neutron momentum. The results of the plateau efficiency,  $\epsilon_{\text{max}}$  are shown in Fig. S25 in red, while the relative fit uncertainty is shown in blue using the second  $y$ -axis.

The veto algorithm will contribute to the inefficiency for neutron detection, since valid neutrons may be detected within the exclusion region of a valid charged particle track or tracklet. We studied the effect of varying the sizes of the exclusion region and merge-windows on the efficiency determination. We chose 50 different combinations of size parameters (from Table S1) and remeasured the neutron efficiency, with results shown in Fig. S26. The variation in efficiency never exceeds 2% of the extracted efficiency. We therefore conservatively assign a 2% relative systematic uncertainty to the efficiency; this uncertainty is small compared to the  $\approx 6\%$  relative uncertainty arising from the fit of the parameterization.

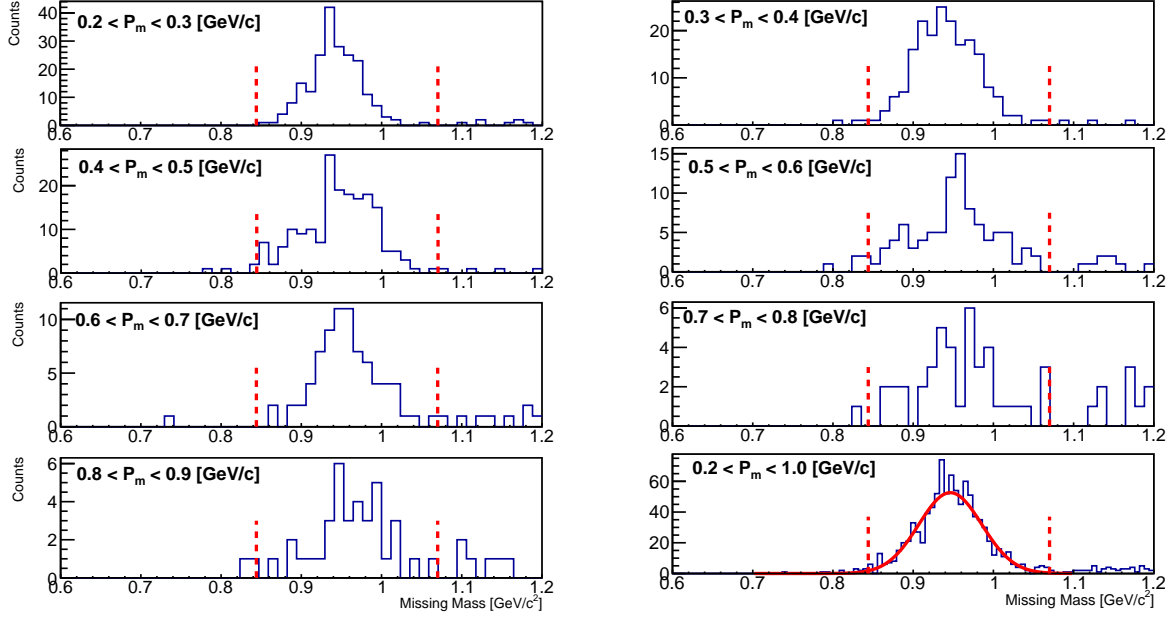

Figure S23: The missing mass (calculated using electron and proton information) for events passing  $d(e, e'pn)$  selection cuts, with the exception of the  $d(e, e'p)n$  missing mass cut, whose range is marked by dotted red lines. The neutron selection cuts largely eliminate background outside the expected missing mass range.

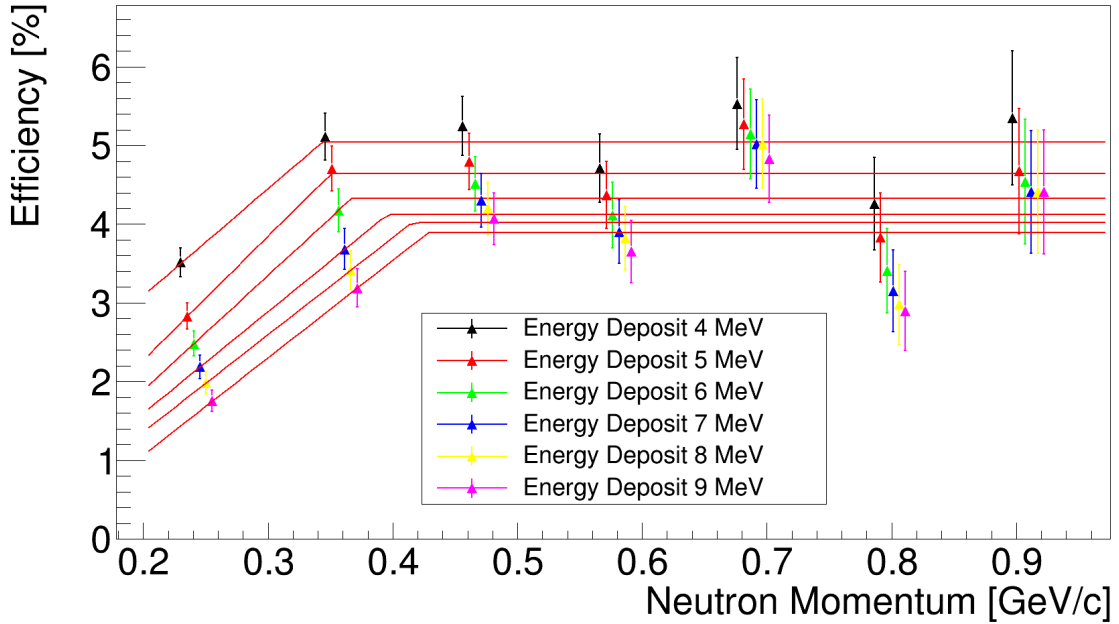

Figure S24: The neutron efficiency for different values of the energy deposition cut. Here, we use missing momentum as a proxy for neutron momentum. The points show the measured efficiency and the red lines show the parameterization of Eq. 6.

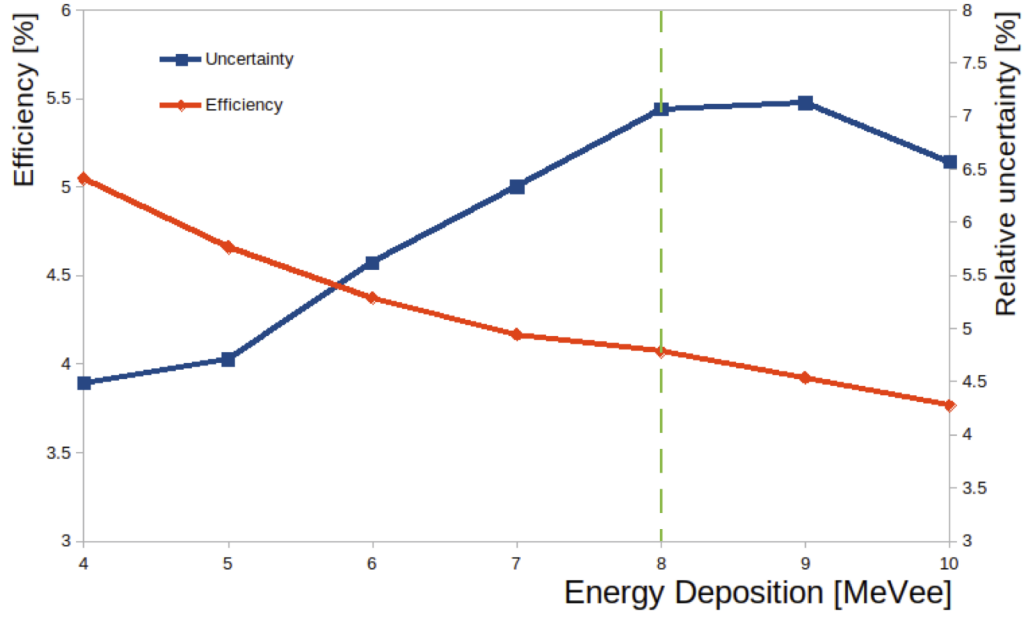

Figure S25: The plateau efficiency as a function of energy deposition cut (red) is shown on the left  $y$ -axis. The relative uncertainty from the fit is shown in blue with  $y$ -axis on the right. The chosen nominal value of 8 MeV for the energy deposition cut is shown as a dashed green line.

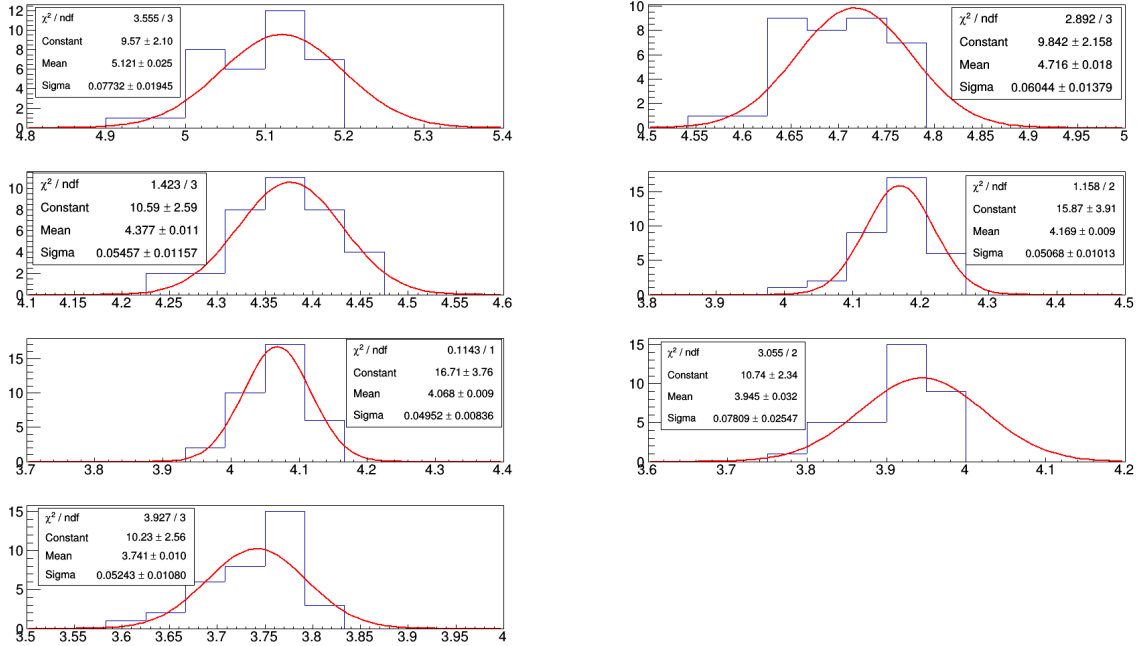

Figure S26: The systematic effect of changing the veto algorithm's exclusion region and merge window sizes, shown for different energy deposition cuts, ranging from 4–10 MeV. Based on these results we choose to apply an additional 2% relative systematic uncertainty to the neutron efficiency.

## 2 Event Selection

### 2.1 $C(e, e'p)$ Event Selection

$C(e, e'p)$  events were selected in kinematics dominated by the break-up of an SRC pair. The event selection criteria were nearly identical to those used in other approved SRC analyses [4–7], in order to permit comparisons of different triple coincidence ratios using the same  $(e, e'p)$  sample. The selection criteria for the  $C(e, e'p)$  sample were:

1. Electron and proton pass fiducial cuts
2. Electron and proton vertices originate from the C target (eliminating background from the deuterium target)
3.  $\theta_{pq} < 25^\circ$
4.  $0.62 < |p_f|/|q| < 0.96$
5.  $x_B > 1.2$
6.  $M_{\text{miss}} < 1.1 \text{ GeV}/c^2$
7.  $0.3 < p_{\text{miss}} < 1.0 \text{ GeV}/c$

Criteria 3 and 4 are used to identify the proton that absorbed the virtual photon, since the proton emerges in the general direction of  $\vec{q}$  with a relatively large fraction of the transferred momentum. Criteria 5 and 6 have the effect of suppressing isobar excitations and selecting high-momentum nucleons in the nuclear ground state. As stated before, the exact values for the cuts were chosen to match those in the  $(e, e'pp)$  analyses of Refs. [4, 6, 7] to allow direct comparison. Criterion 7 restricts the missing momentum to be above the nuclear Fermi momentum ( $\approx 250 \text{ MeV}/c$ ) but below  $1 \text{ GeV}/c$ , where the SRC signal is expected to fall-off relative to the background produced by final-state interactions (matching the upper bound in Refs. [4, 6, 7]). The only difference between these criteria and those used in Ref. [4] are the inclusion of proton fiducial cuts.

### 2.2 $C(e, e'pn)$ Event Selection

We selected  $C(e, e'pn)$  from the sample of  $C(e, e'p)$  events by requiring a neutron hit in the SC passing the veto as well as meeting the following criteria:

- Within the neutron fiducial region (i.e., excluding 10 cm from the ends of all paddles),
- SC energy deposition greater than threshold (nominally 8 MeV),
- Neutron time-of-flight per meter between 4.5 and 9.5 ns/m (corresponding to 0.35–1.0  $\text{GeV}/c$  momentum)

The opening angle between the neutron momentum and  $\vec{p}_{\text{miss}}$  was not considered, since the two vectors are not required to be back-to-back on account of Fermi motion within the nucleus. For the same reason, the neutron's corrected time was also not considered.

Neutrons of interest were selected by looking at the time-of-flight per meter distribution, shown in Fig. S27. A photon peak is clearly visible near the expected value of 3.3 ns/m. There are many events to the left of the photon peak, implying neutral particles travelling faster than light. These events are clearly random background, and give us a good indication of the background levels in the event sample. To the right of the photon peak are the more slowly traveling neutral particles, including the neutrons of interest. Due to the low detection efficiency, and our interest in neutrons from short-range correlated pairs, we limit our analysis to neutrons with momenta greater than 0.35  $\text{GeV}/c$ , corresponding to 9.5 ns/m. To avoid any possible photon contamination, we only consider neutrons with momenta below 1  $\text{GeV}/c$ , corresponding to 4.5 ns/m.

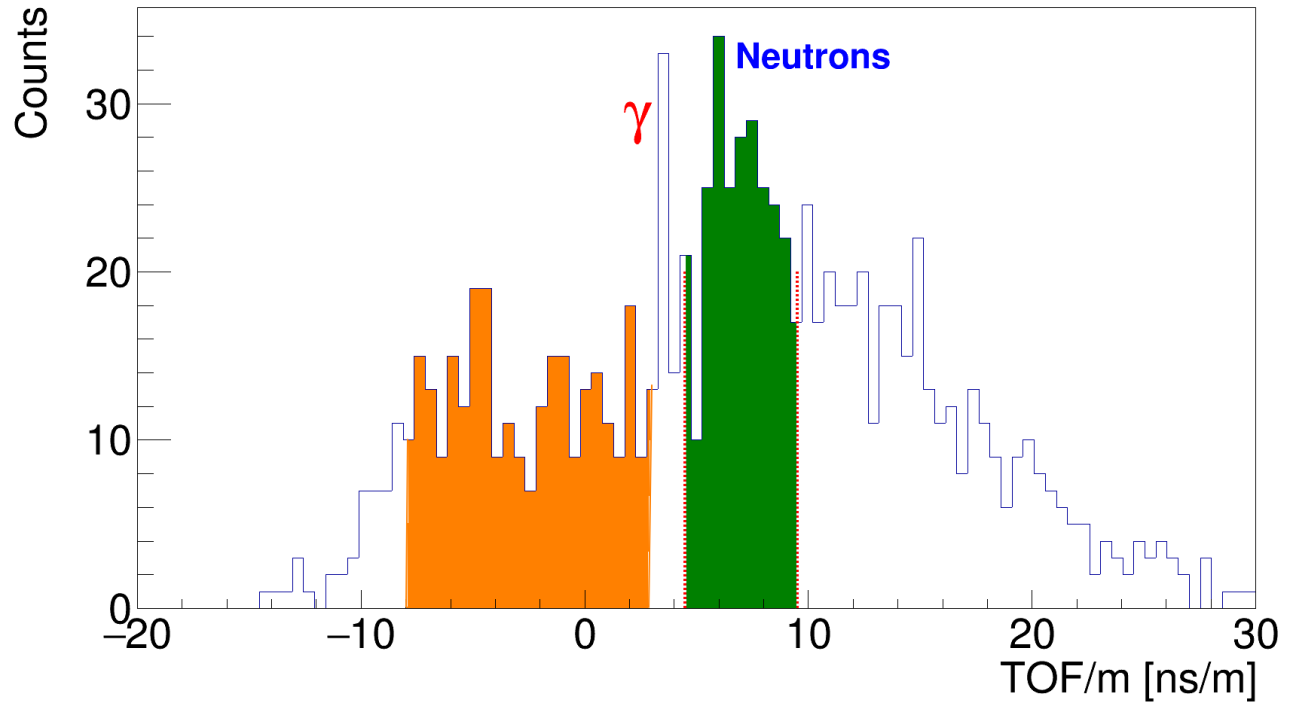

Figure S27: The inverse-velocity distribution (time-of-flight per meter) for  $C(e, e'pn)$  events, with an 8 MeV energy threshold and without any neutron time-of-flight cut. The photon peak, labeled ' $\gamma$ ' is clearly visible at 3.3 ns/m. The neutron signal region, between 4.5 and 9.5 ns/m is shown in green. The region used to determine the background level is shown in orange.

## 2.3 Background Subtraction

The neutron signal sits on top of a large background made up of events in which the neutron candidate is actually random uncorrelated background. This background must be subtracted. Fortunately, since this background is uniformly random in hit time, and therefore uniformly random in inferred time-of-flight, we can use off-time events to estimate the background and subtract it.

To establish the background level per unit time-of-flight, we fit the background region (labeled in orange in Fig. S27) with a constant. Then, for each bin in neutron time-of-flight, we subtract this constant background. The statistical uncertainty estimate for the background-subtracted signal must be updated to reflect Poisson variation of both the signal and background.

With the background level established, we then turn to the spectral shape of the background. When looking at quantities with no dependence on any neutron information, e.g., the missing energy (shown in Fig S28, estimating the spectral shape is relatively simple. We know that the background is drawn from the same underlying distribution as the  $C(e, e'p)$  events in which no neutron was detected. We use the distribution of measured  $C(e, e'p)$  events minus any  $C(e, e'pn)$  events to provide the spectral shape while the fit to off-time neutron events establishes the normalization. Since the number of  $C(e, e'p)$  events is so much larger than the number of  $C(e, e'pn)$  events, there is very little additional statistical uncertainty introduced using this method.

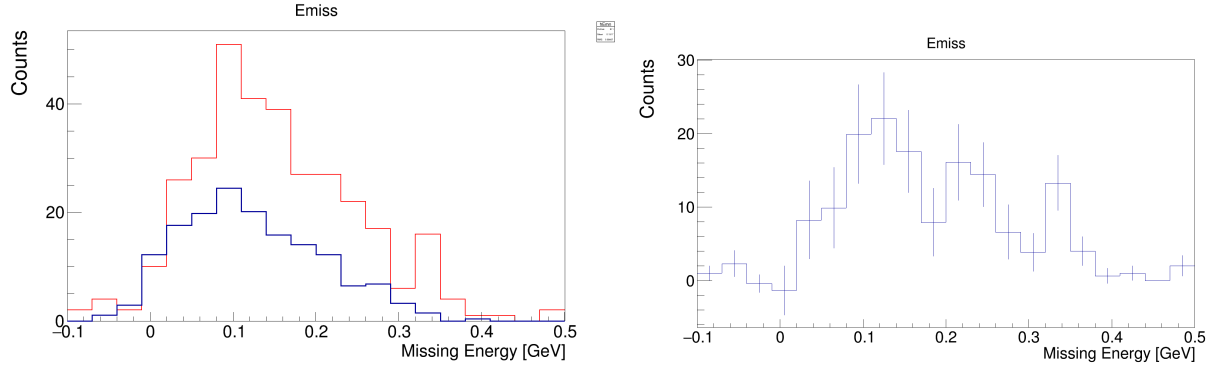

Figure S28: The missing energy spectrum for  $C(e, e'pn)$  events. Left: the signal + background is shown in red while the estimated background spectrum is shown in blue. Right: the signal after background subtraction.

When looking at quantities that depend on neutron hit position information, e.g., the opening angle between  $\vec{p}_{\text{miss}}$  and  $\vec{p}_n$ , we estimate the shape of the background distribution using the off-time neutron events (in the orange background region of Fig. S27). The opening angle distribution of  $C(e, e'pn)$  events is shown in Fig. S29.

## 2.4 Energy Threshold Optimization

To choose the optimal energy threshold for SC hits, we want to balance the goal of maximizing signal with the goal of minimizing background. The figure of merit is the relative statistical uncertainty for the determination of the signal, which, for signal counts  $S$ , and background counts  $B$ , scales as  $\Delta S/S = \sqrt{(S+B)/S}$ . The signal, background, and figure of merit are shown as a function of energy threshold cut in Fig. S30.

As we also want to present results as a function of  $p_{\text{miss}}$ , we want to make sure that our choice of energy threshold cut does not significantly weaken the signal for values of  $p_{\text{miss}}$  with low rate. We divided the  $C(e, e'pn)$  event sample into three regions of  $p_{\text{miss}}$  and looked at the signal and background rates in each as a function of energy threshold cut, shown in Fig. S31. Fortunately, the optimal threshold cut of 8 MeV for the entire sample performs well for each region of  $p_{\text{miss}}$ .

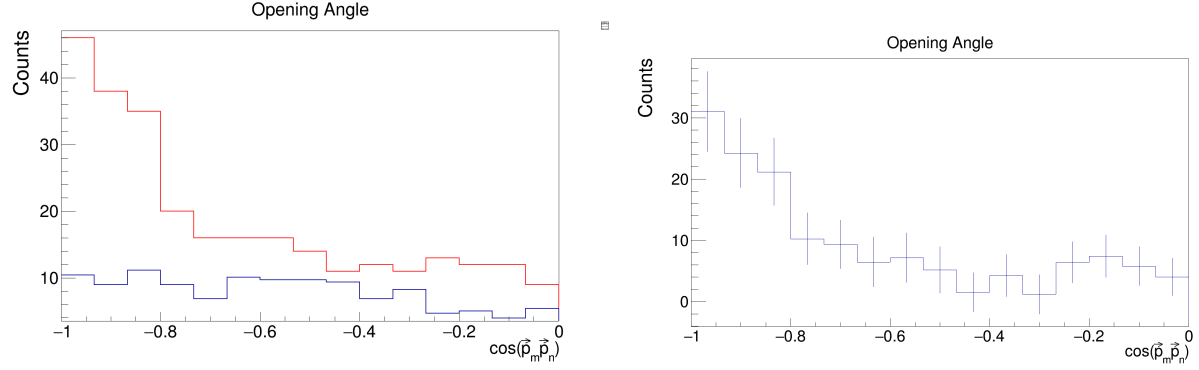

Figure S29: The opening angle spectrum for  $C(e, e'pn)$  events. Left: the signal + background is shown in red while the estimated background spectrum is shown in blue. Right: the signal after background subtraction. The background-subtracted spectrum shows a clear peak at  $180^\circ$ .

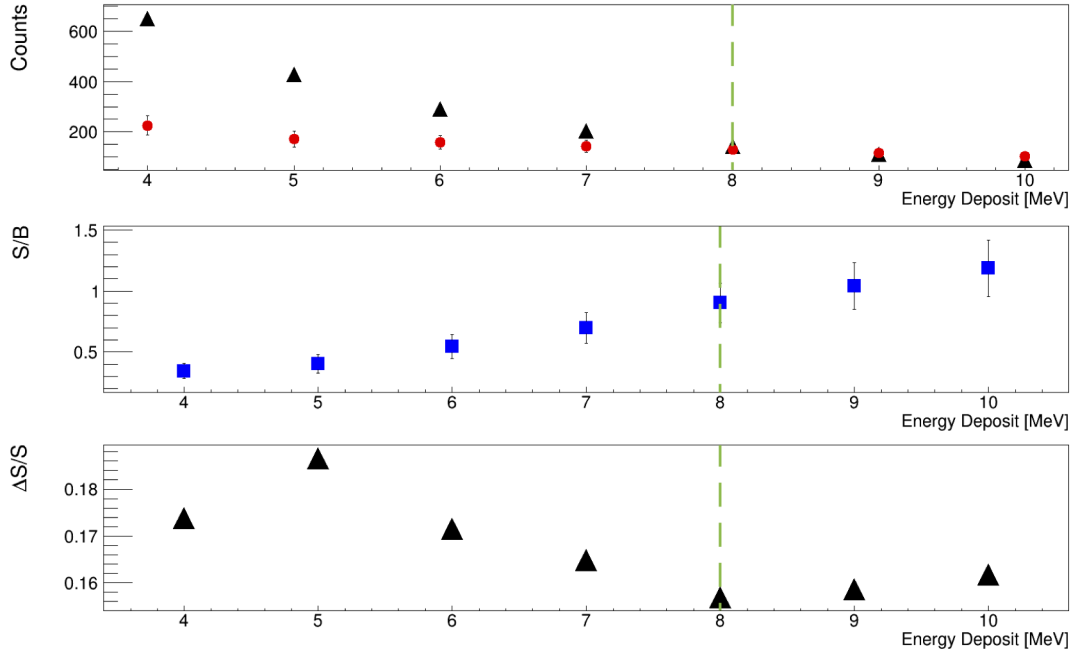

Figure S30: Top: The estimate of the total number of signal  $C(e, e'pn)$  events is shown in red and the estimate of the number of background counts within the signal region is shown in black as a function of energy threshold cut. Middle: signal to background ratio as a function of threshold cut. Bottom: The figure of merit, the relative statistical uncertainty on the determination of the signal as a function of threshold cut. Based on these plots, a threshold cut of 8 MeV was chosen (shown with the green dashed lines).

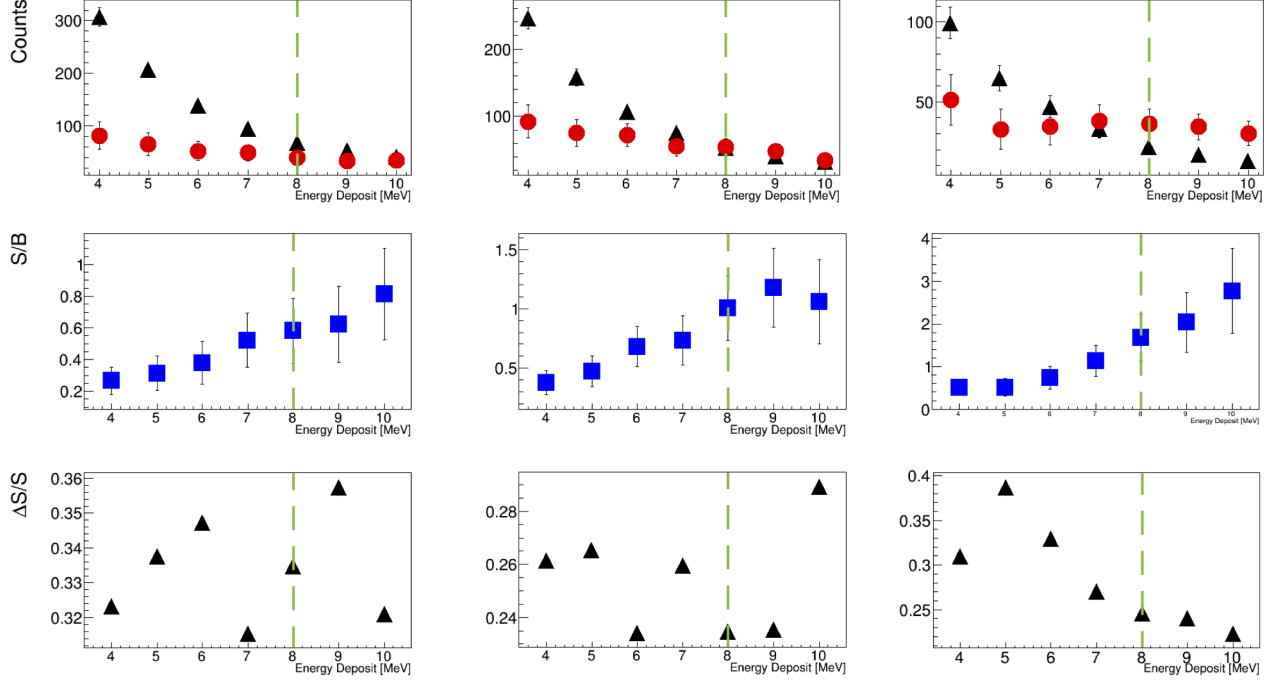

Figure S31: Same as in Fig. S30, but in three different bins of  $p_{\text{miss}}$ . Left column is for  $0.3 < p_{\text{miss}} < 0.45$  GeV/ $c$ . Middle column is for  $0.45 < p_{\text{miss}} < 0.6$  GeV/ $c$ . Right column is for  $0.6 < p_{\text{miss}} < 0.75$  GeV/ $c$ . The green dashed lines show the chosen nominal value of 8 MeV.

Table S3: Uncertainty Budget

| Source                             | 0.3–0.45 GeV/ $c$ Bin | 0.45–0.6 GeV/ $c$ Bin | 0.6–0.75 GeV/ $c$ Bin |
|------------------------------------|-----------------------|-----------------------|-----------------------|
| Neutron efficiency                 | 6.8%                  | 6.8%                  | 6.8%                  |
| Veto algorithm                     | 6.0%                  | 4.0%                  | 6.0%                  |
| Energy deposition cut              | 23%                   | 17%                   | 12%                   |
| Statistics (signal and background) | 31%                   | 25%                   | 25%                   |
| Total                              | 40%                   | 31%                   | 29%                   |

## 2.5 Systematic Uncertainty

In this analysis, as in the previous analysis of Ref. [7], many of the systematic uncertainties affecting data-theory comparisons can only be estimated with model-dependent calculations. Rather than applying model- and theory-dependent corrections to the data, we have left data “as is” wherever possible, and, instead, treated these effects as systematic uncertainties on the theory calculation. However, there are some systematics for which it is clearly more appropriate to assign the uncertainty to the data. These effects include the determination of the neutron efficiency, the effectiveness of the veto algorithm, and the dependence of the results on our specific choice of SC energy deposition cut. Our estimates for the size of these effects on the  $C(e, e'pn)$  yields are shown in Table S3.

The uncertainty from our determination of the neutron efficiency comes from two sources: the fit uncertainty from the constant fit shown in Fig. S24, as well as a 2% relative systematic coming from the use of the charged-particle veto algorithm in the event selection. The two effects lead to a relative uncertainty of 6.8%. The uncertainty on the veto algorithm was estimated by studying the change in yields when varying the sizes of the merge and exclusion windows. The effect on the  $C(e, e'pn)$  yields is  $p_{\text{miss}}$ -dependent. The uncertainty from the choice of energy deposition threshold was determined by studying the sensitivity of the yields to the choice of cut. This is the largest systematic uncertainty on the data. However, as seen in Table S3, the statistical uncertainty is even larger.

Other systematic effects have either been assigned to the theory or are negligible compared to the systematics mentioned above.

## References

- [1] B. A. Mecking *et al.*, “The CEBAF Large Acceptance Spectrometer (CLAS),” *Nucl. Instrum. Meth.*, vol. A503, pp. 513–553, 2003.
- [2] M. D. Mestayer *et al.*, “The CLAS drift chamber system,” *Nucl. Instrum. Meth.*, vol. A449, pp. 81–111, 2000.
- [3] E. S. Smith *et al.*, “The time-of-flight system for CLAS,” *Nucl. Instrum. Meth.*, vol. A432, pp. 265–298, 1999.
- [4] O. Hen, H. Hakobyan, R. Shneor, A. Beck, S. May-Tal Beck, W. Brooks, S. Gilad, I. Korover, E. Piasetzky, and L. Weinst  n, “Probing  $pp$ -SRC in  $^{12}\text{C}$ ,  $^{27}\text{Al}$ ,  $^{56}\text{Fe}$ , and  $^{208}\text{Pb}$  using the  $A(e, e'p)$  and  $A(e, e'pp)$  Reactions,” *CLAS EG2 Analysis Note*, 2012. CLAS Review #7233807.
- [5] M. Duer, E. Piasetzky, O. Hen, E. Cohen, I. Korover, M. Braverman, L. Weinstein, and Khachatryan, “Probing  $pp$ -SRC in  $^{12}\text{C}$ ,  $^{27}\text{Al}$ ,  $^{56}\text{Fe}$ , and  $^{208}\text{Pb}$  using the  $A(e, e'n)$  and  $A(e, e'p)$  Reactions,” *CLAS EG2 Analysis Note*, 2017.
- [6] E. Cohen, M. Duer, E. Piasetzky, O. Hen, and L. Weinstein, “Extracting the center-of-mass momentum distribution of  $pp$ -SRC pairs in  $^{12}\text{C}$ ,  $^{27}\text{Al}$ ,  $^{56}\text{Fe}$ , and  $^{208}\text{Pb}$ ,” *CLAS EG2 Analysis Note*, 2018.
- [7] A. Schmidt, J. Pybus, A. Denniston, A. Hrnjic, E. P. Segarra, F. Hauenstein, M. Khachatryan, M. Duer, E. O. Cohen, E. Piasetzky, L. B. Weinstein, and O. Hen, “Ratio of  $A(e, e'pp)$  to  $A(e, e'p)$  events in SRC kinematics,” *CLAS EG2 Analysis Note*, 2019.
